# Supplementary material for: NeST: Neural Stress Tensor Tomography by leveraging 3D Photoelasticity
Source: arXiv:2406.10212 source file (2024-06-24)
Supplement: Supplementary file 1 [file a2_algorithm_details.tex]

\begin{comment}
\section{Algorithm details}
\subsection{Expression for efficient Jones matrix multiplications}
Here we provide expressions for iteratively accumulating the unique elements of the equivalent Jones matrix, $\mathbf{j}^i_\text{eq}$, as described in Sec.~5.2.
\begin{align}
    a^{i+1}_\text{eq} &= a_ia^{i}_\text{eq} - b_ib^{i}_\text{eq} - c_ic{i}_\text{eq} \\
    b^{i+1}_\text{eq} &= a_ib^{i}_\text{eq} + b_ia^{i}_\text{eq} + c_id{i}_\text{eq} \\
    c^{i+1}_\text{eq} &= a_ic^{i}_\text{eq} + c_ia^{i}_\text{eq} - b_id{i}_\text{eq} \\
    d^{i+1}_\text{eq} &= a_id^{i}_\text{eq} - c_ib^{i}_\text{eq} + b_ic{i}_\text{eq} 
\end{align}
Thus accumulating Jones matrix by just accounting for the unique elements results in 20 multiply-add operations, while a naive complex matrix multiplication of two Jones matrices results in 56 multiply-add operations.
\subsection{\texttt{Two-step} approach implementation}
\end{comment}
% \ad{Pseudo-code}
% \ad{Details of the Two-step techniqu}
